# Supplementary material for: GAF: Gaussian Avatar Reconstruction from Monocular Videos via Multi-view Diffusion
Source: arXiv:2412.10209 source file (2025-04-14)
Supplement: Supplementary file 1 [file additional_figure.tex]

\begin{figure*}[t]
    %\vspace{-3mm}
    \centering
    \includegraphics[width=\linewidth]{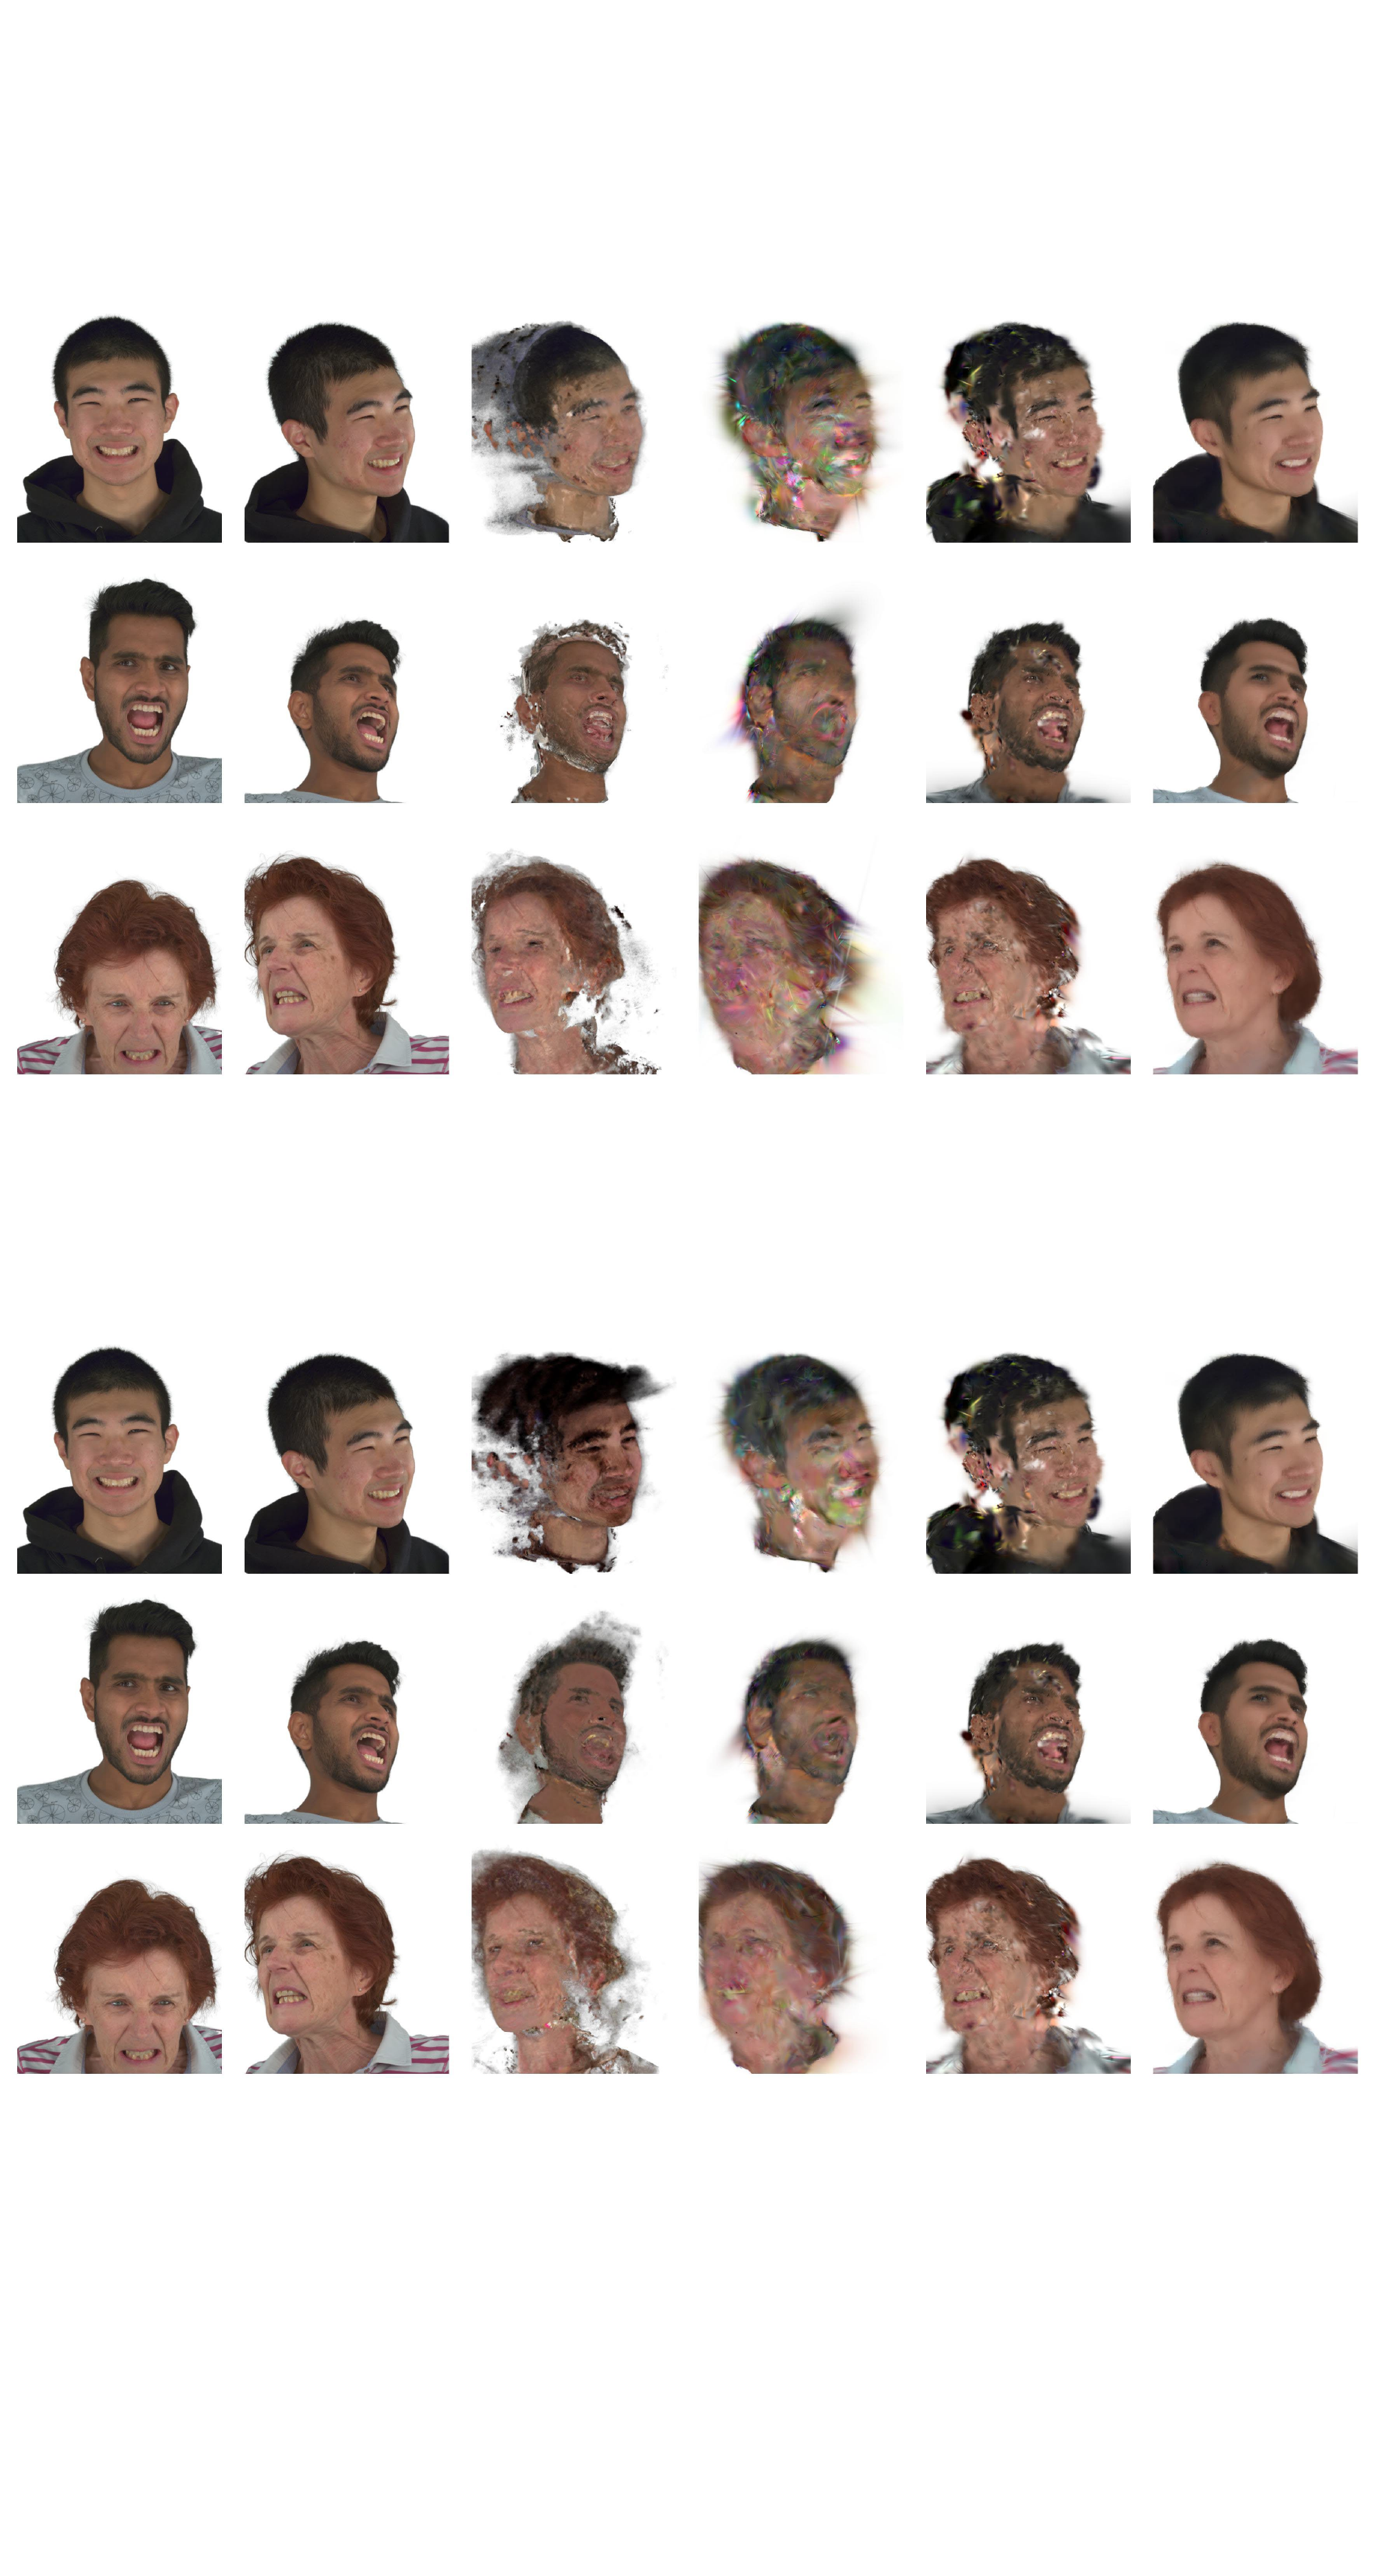}
    \begin{tabular*}
        {\linewidth}{
            @{\extracolsep{\fill}}
            p{0.13\linewidth}
            p{0.11\linewidth}
            p{0.13\linewidth}
            p{0.15\linewidth}
            p{0.10\linewidth}
            p{0.16\linewidth}
        }
        \centering (a) Input frame
        & \centering (b) INSTA
        & \centering (c) FlashAvatar
        & \centering (d) GaussianAvatars
        & \centering (e) Ours
        & \centering (f) Ground truths\\
    \end{tabular*}
    \vspace{-4mm}
    \caption{\textbf{Novel view synthesis from monocular videos on the Nersemble dataset.} Compared to state-of-the-art methods, our method consistently produces more favorable renderings from both near and far hold-out views, and captures more accurate facial expression details.}
    \label{fig:novelview}    
\end{figure*}
\begin{figure*}[h]
    \centering
    \includegraphics[width=.9\linewidth]{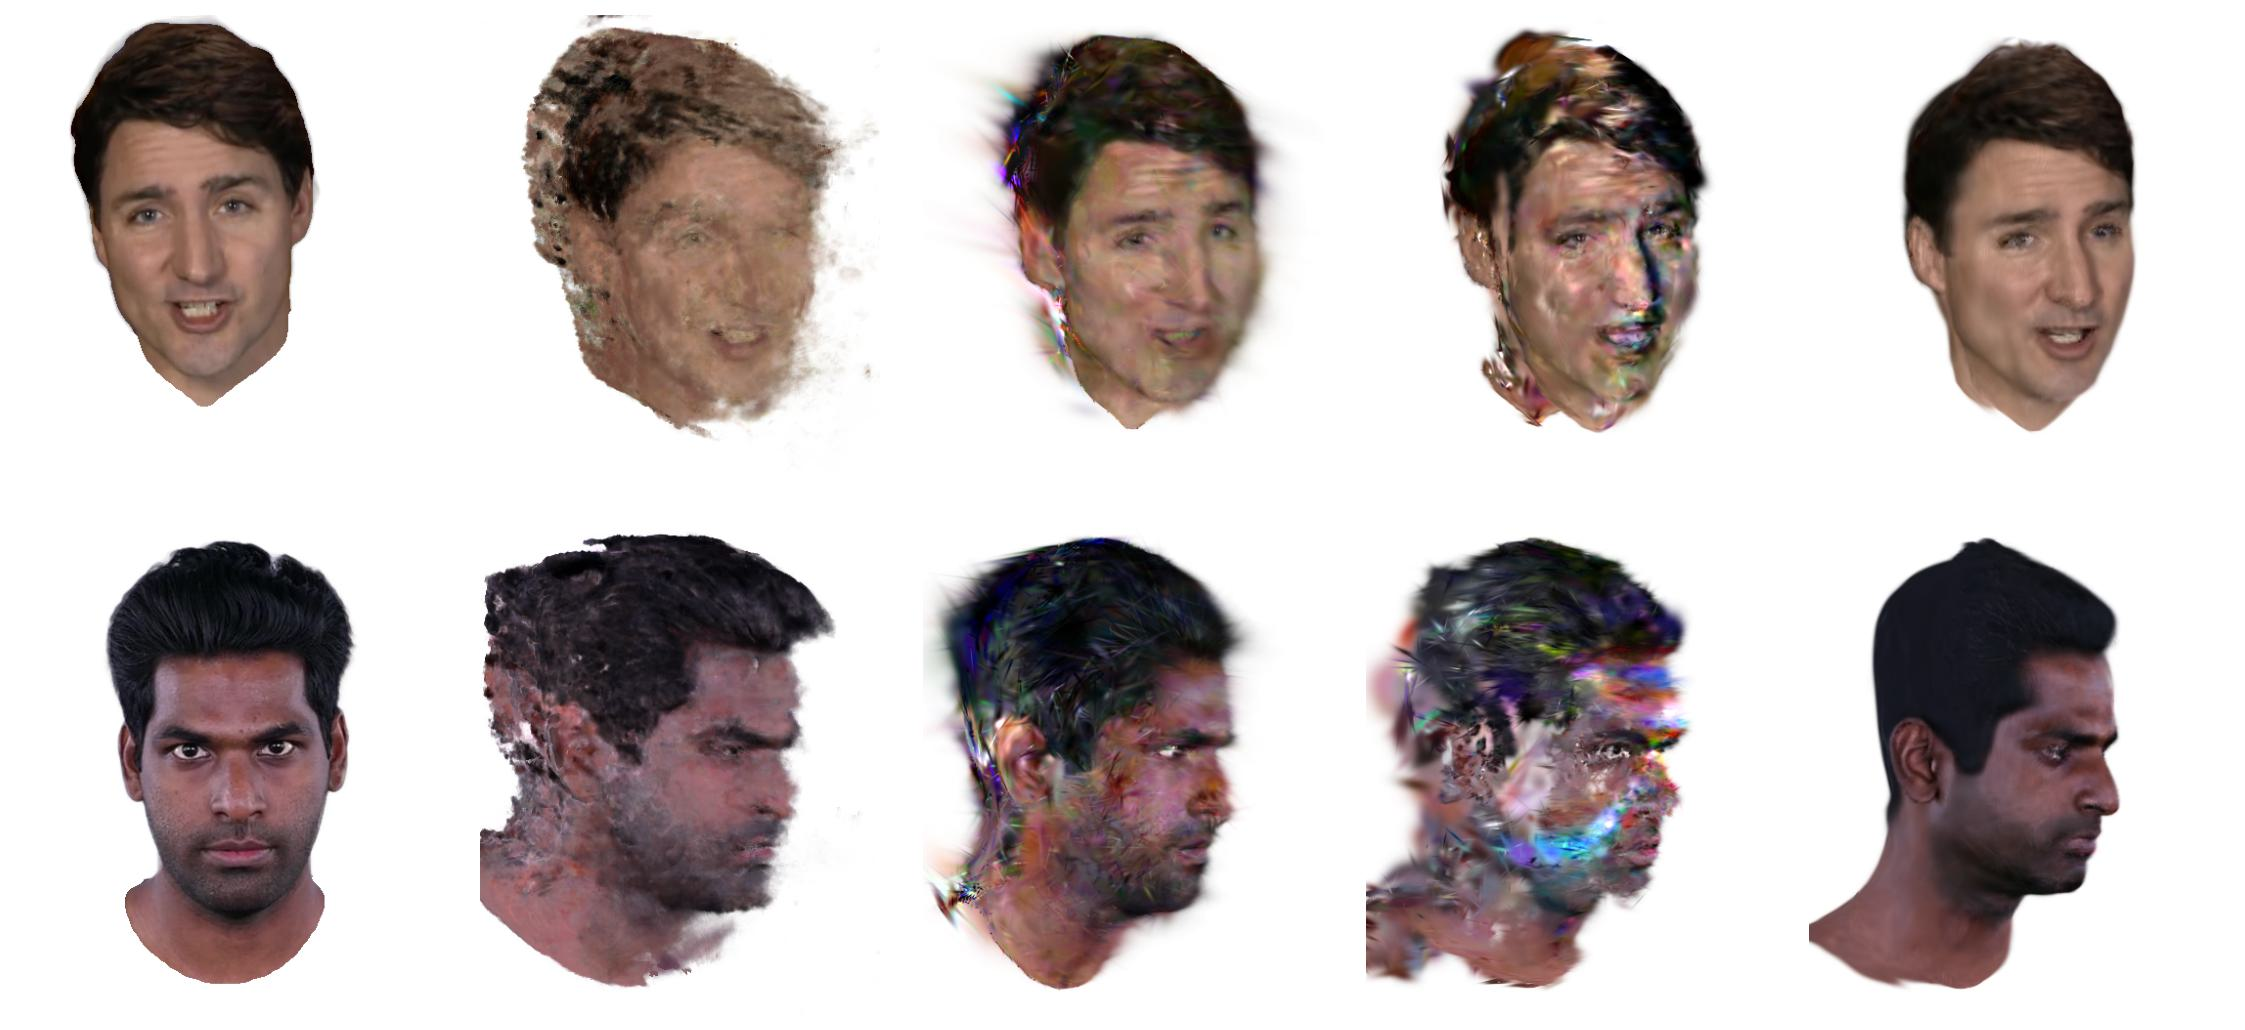}
    \begin{tabular*}{\linewidth}{@{\extracolsep{\fill}}p{0.07\linewidth}p{0.12\linewidth}p{0.15\linewidth}p{0.15\linewidth}p{0.15\linewidth}p{0.15\linewidth}p{0.10\linewidth}p{0.20\linewidth}}
    \centering & (a) Input frame & \centering (b) INSTA & \centering (c) FlashAvatar & \centering (d) GaussianAvatars & \centering (e) Ours & \\
    \end{tabular*}
    \caption{\textbf{Novel view synthesis on in-the-wild monocular videos.} Given a sequence captured from the front view, our approach can still generate photo-realistic novel-view renderings, even from an extreme side view (bottom). However, existing methods fail to extrapolate to this case.}
    \label{fig:novelview_real}
\end{figure*}

\begin{figure*}[!htp]
    \centering
    \includegraphics[width=\linewidth]{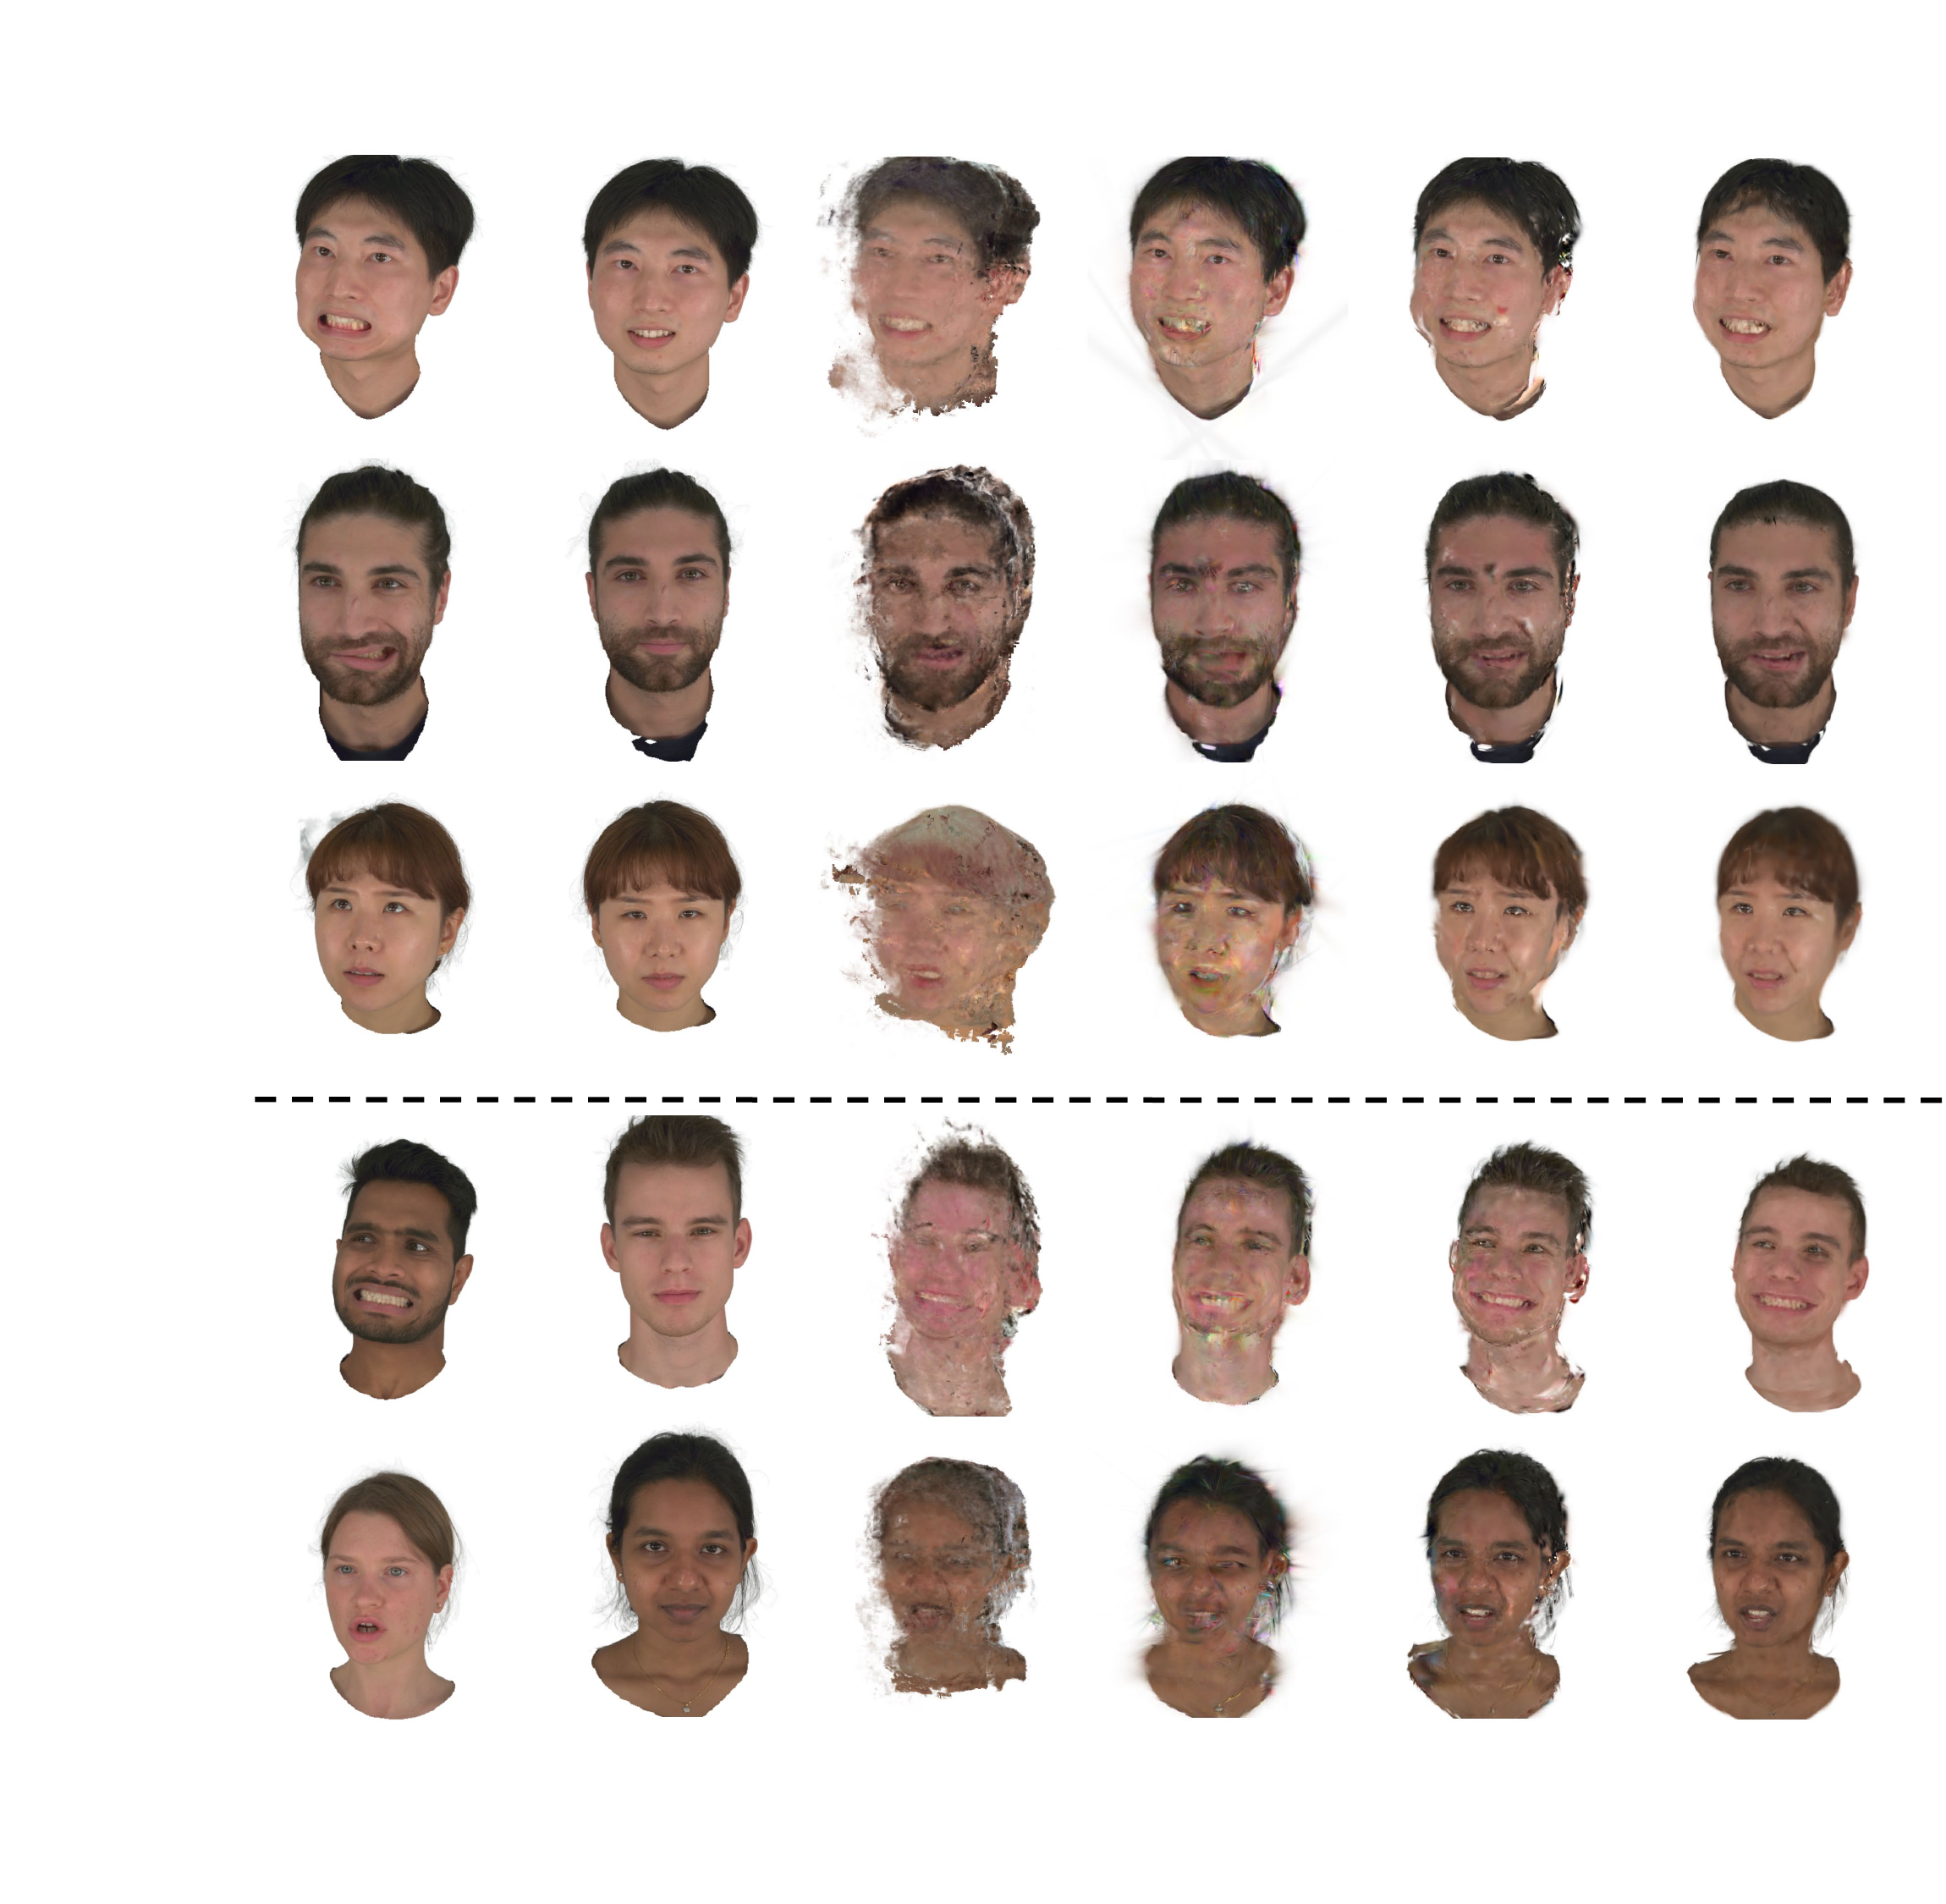}
    \begin{tabular*}{\linewidth}{@{\extracolsep{\fill}}p{0.15\linewidth}p{0.15\linewidth}p{0.15\linewidth}p{0.15\linewidth}p{0.15\linewidth}p{0.15\linewidth}p{0.15\linewidth}}
    \centering (a) Driving frame & \centering (b) Source Identity & \centering (c) INSTA & \centering (d) FlashAvatar & \centering (e) GaussianAvatars & \centering (f) Ours \\
    \end{tabular*}
    \vspace{-6mm}
    \caption{\textbf{Self Reenactments from Monocular videos on the Nersemble dataset.}
    We use the tracked FLAME pose and expressions of a driving sequence to animate the reconstructed Gaussians.
    Our method demonstrates better generalization ability to novel expressions and produces higher quality novel views.
    }
    \label{fig:selfnact}
\end{figure*}
\begin{figure*}[!htp]
    \centering
    \includegraphics[width=\linewidth]{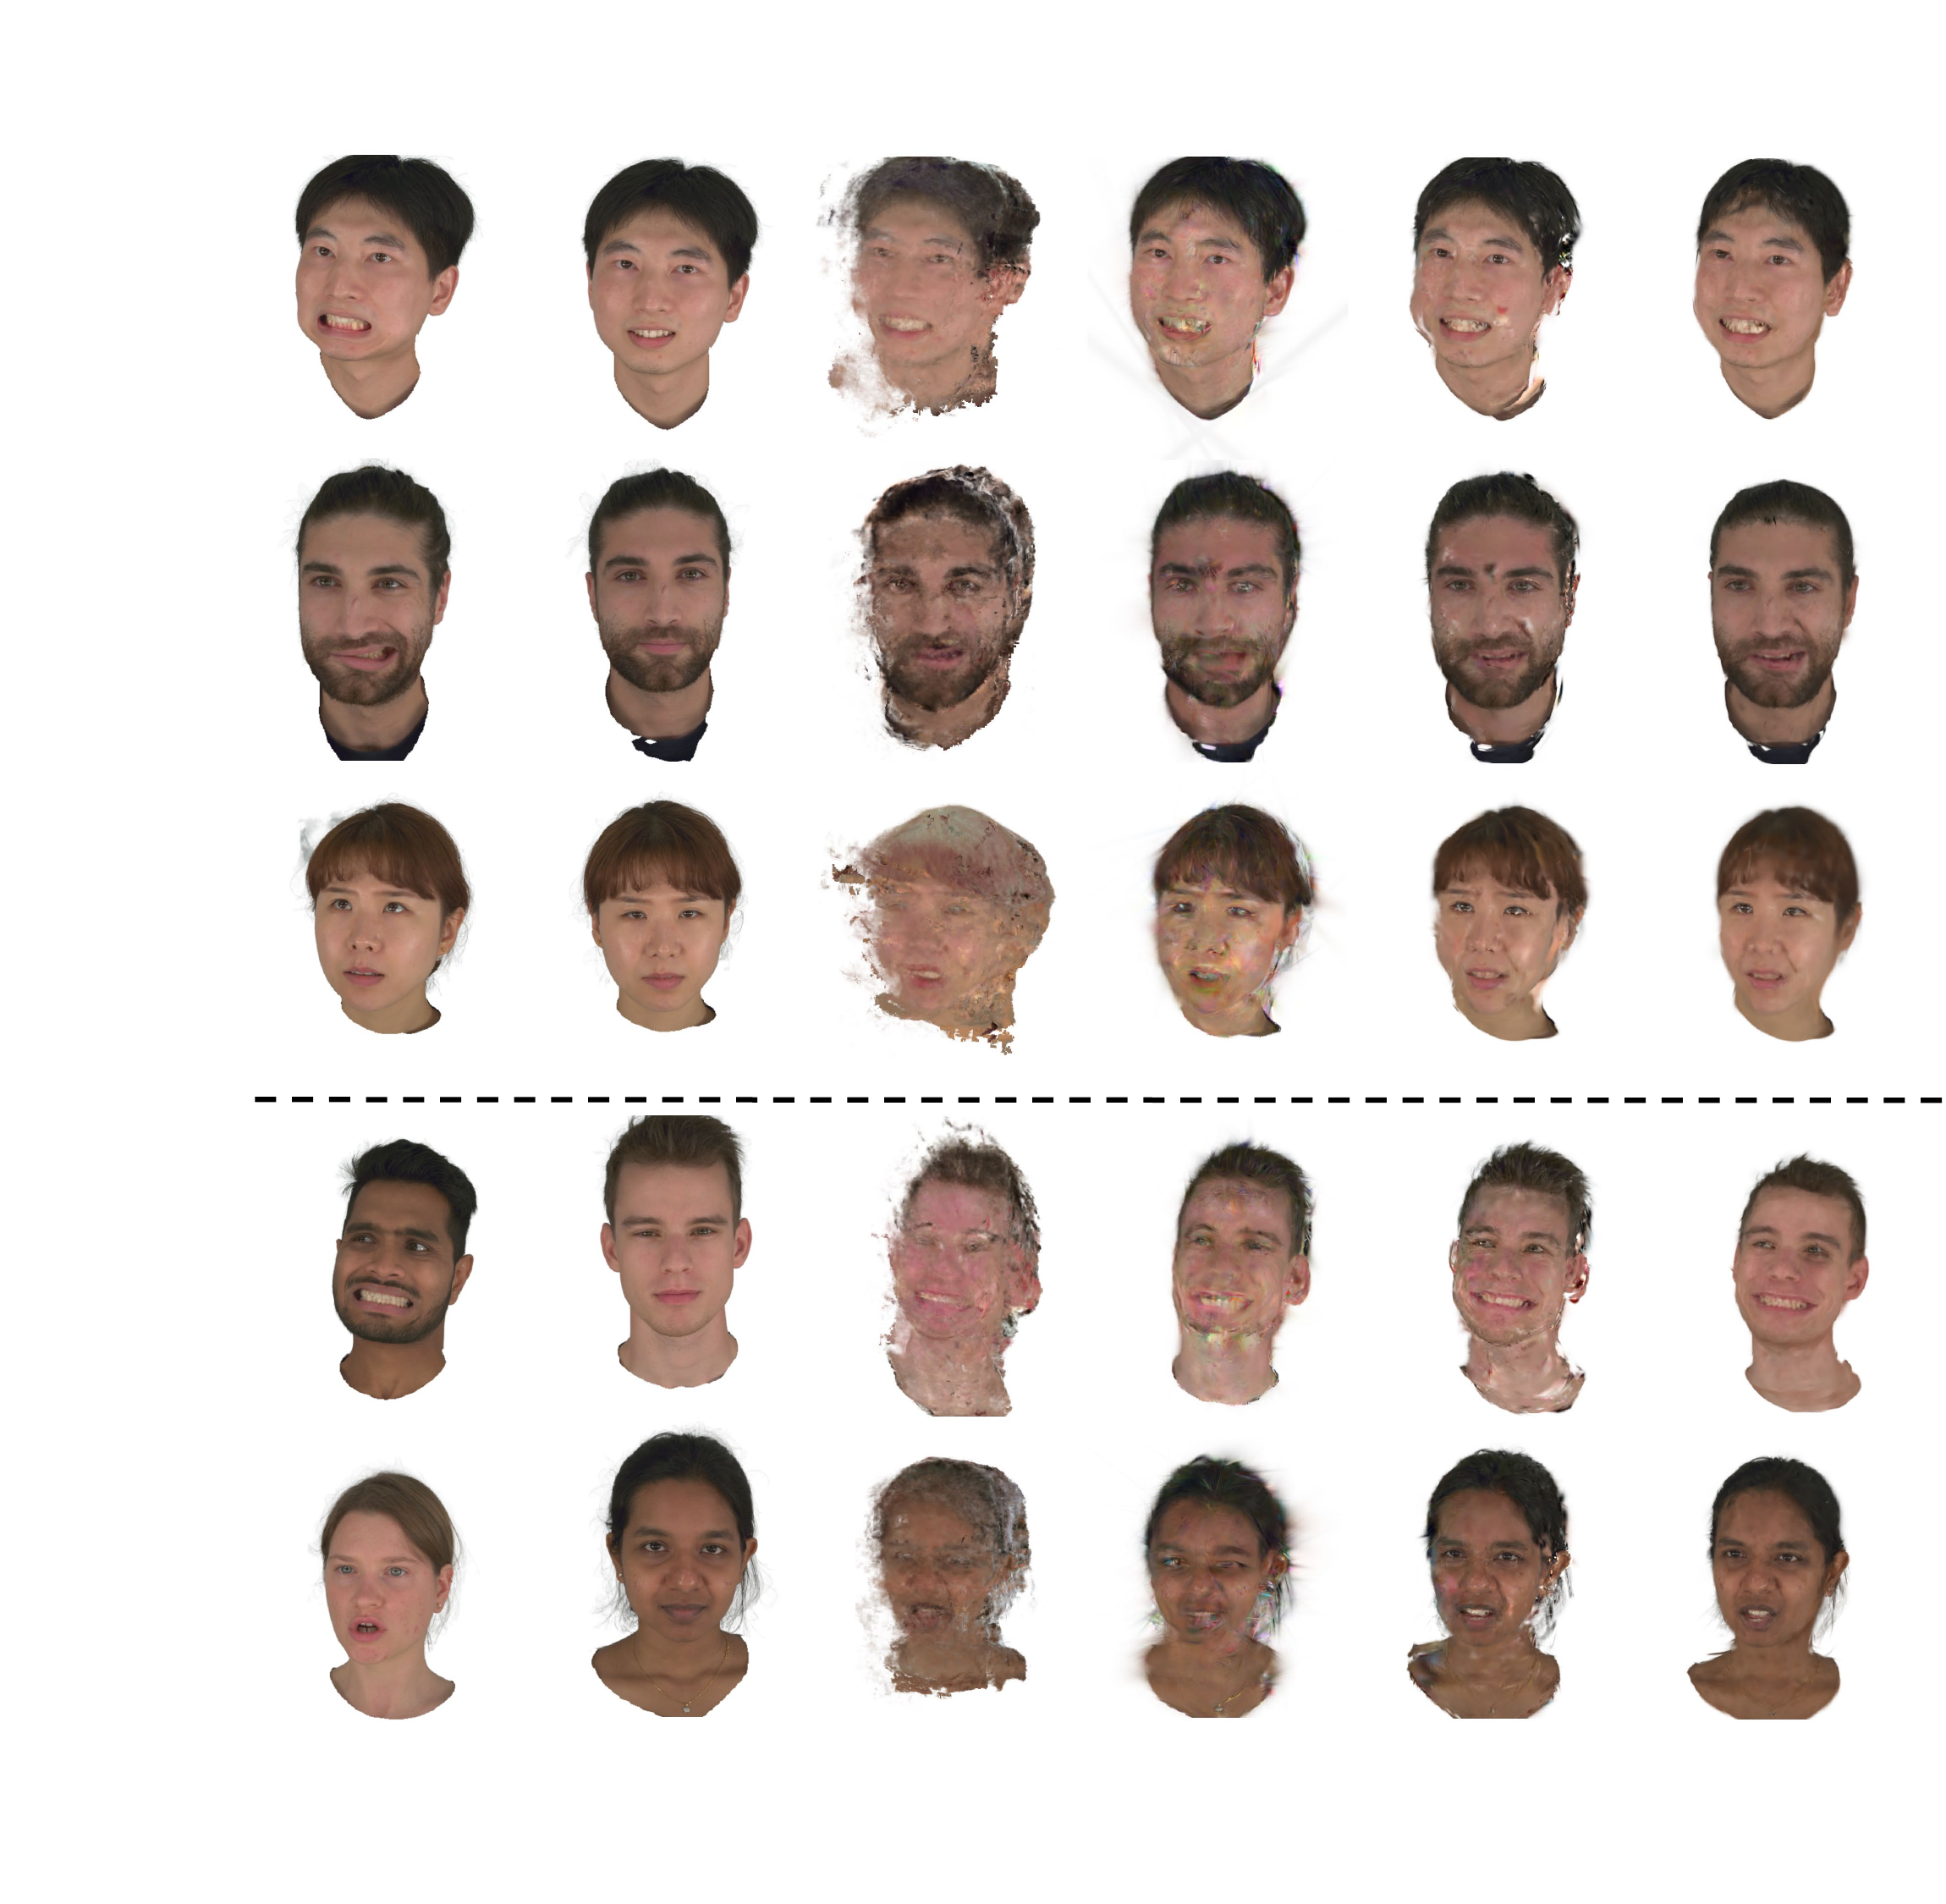}
    \begin{tabular*}
        {\linewidth}{@{\extracolsep{\fill}}p{0.15\linewidth}p{0.16\linewidth}p{0.13\linewidth}p{0.16\linewidth}p{0.14\linewidth}p{0.16\linewidth}p{0.09\linewidth}}
        \centering (a) Driving frame & \centering (b) Source Identity & \centering (c) INSTA & \centering (d) FlashAvatar & \centering (e) GaussianAvatars & \centering (f) Ours \\
    \end{tabular*}
    \vspace{-6mm}
    \caption{\textbf{Cross-Reenactments from Monocular videos on the Nersemble dataset.} 
    Our method outperforms state-of-the-art methods by showcasing more vivid expression transfers and more plausible renderings around the mouth region.}
    \label{fig:crossnact}
\end{figure*}
